# Supplementary material for: Higher Order Kernel Mean Embeddings to Capture Filtrations of Stochastic Processes
Source: arXiv:2109.03582 source file (2021-11-04)
Supplement: Supplementary file 1 [file appendix_split.tex]

\documentclass[letterpaper]{article}

\usepackage{pdfpages}

\usepackage{bashful}

\begin{document}

\bash
latexmk -pdf main >& /dev/null
\END

\includepdf[pages=14-23]{main}

\end{document}
